# Supplementary material for: High-Fidelity Single-Qubit Gates for Two-Electron Spin Qubits in GaAs
Source: arXiv:1404.1712 ancillary file (2021-01-22)
Supplement: Supplementary file 1 [file Supplement.pdf]

# Supplementary Material: High-Fidelity Single-Qubit Gates for Two-Electron Spin Qubits in GaAs

Pascal Cerfontaine[1],* Tim Botzem[1], David P. DiVincenzo[1, 2], and Hendrik Bluhm[1]
[1]*JARA-Institute for Quantum Information, RWTH Aachen University, D-52074 Aachen, Germany and*
[2]*Peter Grünberg Institute: Theoretical Nanoelectronics, Research Center Jülich, D-52425 Jülich, Germany*
(Dated: April 7, 2014)

This supplemental information is organized as follows: In the first section, further details regarding the numerical fidelity optimization will be presented, including a more in-depth discussion of the resulting pulse sequences. In the second section, we will focus on the self-consistent calibration routine.

## CONTENTS

I. Fidelity optimization 1
- A. Transfer function $J(\epsilon)$ 1
- B. Noise model 1
- C. Optimization problem 2
- D. Externally varied parameters 2
- E. Idle axis concept 2
- F. Rabi interpretation 3
- G. Mechanisms for high fidelities 3
- H. Further solutions 4
- I. Noise contributions 4
- J. Gate robustness to model errors 4
- K. Numerical analysis 5

II. Self-consistent calibration routine 8
- A. Choice of weights 8
- B. Measurement noise 9
- C. Convergence 9
- D. Fidelity $\mathcal{I}_{\mathrm{sys}}$ 9
- E. Setting the orientation of the rotation axes in the $xy$-plane 10

References 10

## I. FIDELITY OPTIMIZATION

A detailed introduction to the perturbative method we use to obtain first-order filter functions of an arbitrary quantum gate is given in [1, 2]. The filter function obtained in this way is then used to calculate the gate fidelity under the influence of fast non-Markovian charge noise. Slow noise sources are taken into account by sampling in discrete intervals from a Gaussian distribution. Our implementation is fast enough for numerical optimization and sufficiently accurate for the experimental noise levels used in this work. We checked all fidelities calculated with this fast method against the results of Monte Carlo simulations of the qubit's time evolution and found the relative error to be usually below 15%, well within other uncertainties of our physical qubit model. Energy relaxation was neglected in this work, as the associated timescale $T_1$ is in excess of 100 µs [3], much longer than gate sequences and $T_2^\star$.

### A. Transfer function $J(\epsilon)$

Parameters for the phenomenological model $J(\epsilon) = J_0 \exp(\epsilon/\epsilon_0)$ were fitted from data measured by Dial *et al.* [3] to $J_0 = 1\,\mathrm{ns}^{-1}$ and $\epsilon_0 = 0.272\,\mathrm{mV}$ (the angular frequency $J_0$ corresponds to a frequency $J_s = 159\,\mathrm{MHz}$). In the numerical optimization, the detuning was constrained to $-5\epsilon_0 < \epsilon < 5\epsilon_0$ and in the last 4 ns of each pulse $\epsilon$ was set to $\epsilon_{\mathrm{min}} = -5\epsilon_0$ to avoid transients. Rise times were modeled as exponential $\propto \exp(-t/\tau_{\mathrm{rise}})$ with $\tau_{\mathrm{rise}} = 1\,\mathrm{ns}$. In order to integrate the Schrödinger equation, we approximate pulse shapes as piecewise constant. Specifically, we subdivide each 1 ns bin (green in Fig. 2) into 5 smaller bins (black). We could have performed piecewise linear integrations [4], but the complexity of the integration steps was not deemed worth the effort.

### B. Noise model

All our calculations are based on a Hamiltonian which includes random variables $\delta\epsilon$ and $\delta\Delta B_z$ representing classical hyperfine and charge noise

$$H = \frac{J(\epsilon(t) + \delta\epsilon(t))}{2}\sigma_z + \frac{\Delta B_z + \delta\Delta B_z}{2}\sigma_x \tag{S.1}$$

$$\approx \frac{J(t)\cdot(1 + \delta\epsilon(t)/\epsilon_0)}{2}\sigma_z + \frac{\Delta B_z + \delta\Delta B_z}{2}\sigma_x, \tag{S.2}$$

where we have expanded the phenomenological model $J(\epsilon) = J_0 \exp(\epsilon/\epsilon_0)$ up to first order in the small noise term $\delta\epsilon$. One can easily see that the effect of charge noise noise $\delta\epsilon$ depends directly on the level of the control amplitude $J$ which makes high exchange energies $J$ unattractive for reaching high fidelities.

We use experimentally determined noise models for both random variables. Since gates are performed on

* cerfontaine@physik.rwth-aachen.de

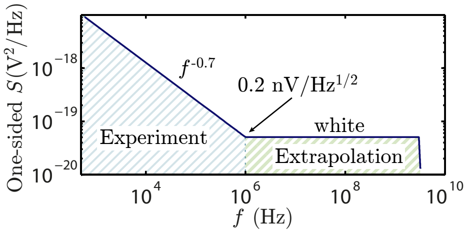


FIG. S.1. Measured charge noise spectrum [3] and conservative extension to high-frequency regions of interest for fast qubit gates.

a ns timescale, hyperfine fluctuations with main spectral weight below 10 Hz can be modeled as quasistatic. For stabilized hyperfine gradients (using dynamic nuclear polarization), each time a quantum gate is performed, a different offset $\delta\Delta B_z$ from a Gaussian distribution with $\sigma_{\Delta B_z} \approx 0.5\,\mathrm{mT}$ can be used to describe the noise [5]. In contrast to hyperfine noise, charge noise can only be partially described as quasistatic. Its high-frequency part is best captured using (two-sided) spectral noise densities $S^t_\epsilon(\omega)$ defined as the Fourier-transform of the correlation function of a time-dependent variable $c(t)$ like

$$S^t_c(\omega) = \int_{-\infty}^{\infty} \langle c(t)\cdot c(t+\Delta t)\rangle\, e^{-i\omega t}\, dt. \tag{S.3}$$

Unless otherwise noted, we use one-sided spectral densities $S_c(\omega) = 2S^t_c(\omega)$. From echo amplitude decays, Dial *et al.* [3] extracted $S_\epsilon(f) = 8\times 10^{-16}\frac{\mathrm{V}^2}{\mathrm{Hz}}\left(\frac{\mathrm{Hz}}{f}\right)^{0.7}$ from 50 kHz to 1 MHz, with a standard deviation $\sigma_\epsilon = 8\,\mu\mathrm{V}$ which includes slow noise. Since qubit gates on a ns timescale are most sensitive to fluctuations above 1 MHz, we conservatively extend the spectrum as white above 1 MHz until 3 GHz, which is shown in Fig. S.1. The upper cutoff of 3 GHz was chosen as low as possible for computational efficiency but high enough not to influence the calculated effects of $\epsilon$-noise on gate performance.

### C. Optimization problem

Overall, there are three different types of noise present in the system, namely fast $\epsilon$-noise, quasistatic $\epsilon$-noise and $\Delta B_z$-noise. We calculate the contribution to the total infidelity of each of these noise sources separately because our noise levels are sufficiently small so that interaction effects are negligible. We apply the perturbative method [1, 2] only for the fast $\epsilon$-component and sample from a two-dimensional Gaussian distribution for both quasistatic noise terms. The perturbative method converges because the expansion coefficient $\sigma_{\epsilon,\mathrm{fast}}\tau/2 \ll 1$ for the noise levels and gate durations $\tau$ used in our work.

We combine the different contributions to $\mathcal{I}$ into a vector as given in Eq. 1. Because our objective is to find gates with optimal noise properties but negligible systematic error, we additionally include the components $\boldsymbol{\Delta}(\boldsymbol{\epsilon}) = \phi(\boldsymbol{\epsilon})\boldsymbol{n}(\boldsymbol{\epsilon}) - \phi_t \boldsymbol{n_t}$. Given sufficient degrees of freedom ($N_\mathrm{seg}$ large enough) it is not very hard to remove systematic errors starting from random initial $\boldsymbol{\epsilon}$. Therefore, minimizing the sum of squares of the objective vector valued function (as given in Eq. 1) typically produces results where the three components of $\boldsymbol{\Delta}$ are smaller than $\mathcal{I}_{\Delta B_z}(\boldsymbol{\epsilon})$, $\mathcal{I}_{\epsilon,\mathrm{slow}}(\boldsymbol{\epsilon})$ and $\mathcal{I}_{\epsilon,\mathrm{fast}}(\boldsymbol{\epsilon})$. Since the unitary infidelity $\mathcal{I}_U$ (which describes systematic errors) from a systematic overrotation by an angle $\phi$ is proportional to $\phi^2$ [6], this leads to a much smaller $\mathcal{I}$ from systematic errors (usually on the order of $10^{-10}$) than from the different noise contributions (about $10^{-3}$ to $10^{-4}$).

### D. Externally varied parameters

In principle, the number of $\epsilon$-segments $N_\mathrm{seg}$ is also a parameter which could be optimized directly. However, this is harder to incorporate into the optimization since it can only take on discrete values. Additionally, we prefer short solutions for straightforward experimental implementation. Therefore, we varied the number of $\epsilon$-segments externally while keeping them as low as possible. If the duration of one segment is fixed, the resulting gate sequences will therefore have discrete gate lengths $T$ determined by $N_\mathrm{seg}$.

For single qubit operation (i.e. for dynamical decoupling or quantum process tomography), it will be necessary to concatenate several quantum gates. If all gates have the same duration $T$ this provides the quantum system with a clock rate similar to classical computers. It might also be convenient to just retain the current qubit state over one clock cycle period. This is most easily done by (almost) pure $\Delta B_z$-rotations with $\sqrt{\Delta B_z^2 + J(\epsilon_\mathrm{min})^2}\,T = 2\pi N_{\Delta B_z}$, $N_{\Delta B_z} \in \mathbb{N}$, where $N_{\Delta B_z}$ gives the number of pure $\Delta B_z$-rotations and the exchange splitting is kept constant at $J(\epsilon_\mathrm{min}) = J_\mathrm{min} \ll \Delta B_z$. Since noise in $\Delta B_z$ is slow, it is possible to use gates to perform dynamical decoupling if it is desired to keep the quantum state alive for several clock periods. The concept of using pure $\Delta B_z$-rotations to retain the qubit state over a clock cycle $T$ leads to discrete $\Delta B_z$-values, which can be characterized by the number of rotations $N_{\Delta B_z}$ in one clock cycle period or "idle period" (if $J = J_\mathrm{min}$). Like $T$, these discrete $\Delta B_z$-values can be varied externally in numerical optimization. Since high $N_{\Delta B_z}$ are unattractive because of increased relaxation during readout [7], we only consider low $N_{\Delta B_z}$.

### E. Idle axis concept

In the main text we only presented solutions for gates around the $x$- and $y$-axis. In order to motivate and easily describe additional gates for which we carried out the optimization, we will now introduce a new reference frame.

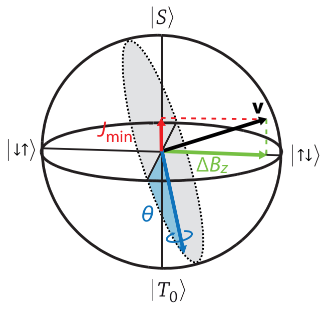


FIG. S.2. Target gates create rotations around axes (dark blue), which lie in the idle plane (grey). The plane's normal vector $\boldsymbol{v}$ (black) is given by $(\,\Delta B_z,\ 0,\ J_{\mathrm{min}}\,)^T$. The rotation axes of different gates are then completely characterized by $\boldsymbol{v}$ and a rotation in this plane given by $\theta$ (light blue).

In the following we will refer to the axis defined by $\Delta B_z$ and $J_{\mathrm{min}}$ as the "idle axis", shown in black in Fig. S.2. As this is the axis $\boldsymbol{v}$ around which the qubit precesses if no control pulses in $\epsilon$ are applied (when $\epsilon$ is kept constant at $\epsilon_{\mathrm{min}}$), it is natural to define this as the $z$-axis in a rotated frame of reference, from now on denoted by $z'$. By rotating around the idle axis for fractions of $T$, phase gates around $z'$ can be carried out in a very straightforward manner in an experiment. Furthermore, the idle axis defines an "idle plane", which is very close to the $yz$-plane. Gates around axes orthogonal to $z'$ lie in this idle plane and correspond to $x'$- and $y'$-gates in this coordinate system. We therefore searched for gates which rotate around orthogonal axes in the idle plane. Each gate's rotation axis can be described by an angle $\theta$, as illustrated in blue in Fig. S.2, with the convention that $\theta = 0$ is the negative $y$-axis in the original reference frame.

### F. Rabi interpretation

As mentioned in the main text, the solutions of the minimization problem in Eq. 1 can be interpreted as Rabi oscillations, which are corrected for the experimental constraints, work without a rotating wave approximation and honor $J > 0$ by excluding the negative half-waves. This is shown explicitly in Fig. S.3, where solutions for $\pi/2$-gates around different rotation axes are shown. All of the rotation axes lie in the idle plane. The state vector rotates by approximately $2\pi$ in between two $J$-pulses. Furthermore, the pulses are phase-shifted with respect to each other. Similar to Rabi driving, this realizes rotations around different axes. The Rabi interpretation also explains why the number of pulses usually goes up as $N_{\Delta B_z}$ is increased, namely because the state vector executes $2\pi$ rotations much faster. Solutions typically have as many peaks in $J$ as $N_{\Delta B_z}$, except for rotation axes where the phase shift is just right to be able to fit an additional pulse (as seen for example in the pulse on the top).

### G. Mechanisms for high fidelities

One method for reaching high fidelities is to keep $J$ as low as possible while still realizing the target gate (see main text). This leads to lower infidelities from the slow and fast charge noise components. However, the slow components in $\epsilon$ and $\Delta B_z$ can also be reduced by dynamical error cancellation, similar to dynamical decoupling techniques like spin echo. This approach is explicitly exploited in dynamically corrected gates (DCGs) [8–10] where the first-order derivatives of the time evolution operator with respect to changes in $\epsilon$ and $\Delta B_z$ are set to zero, making them first-order insensitive to slow noise.

While the (matrix) 2-norm of both first-order derivatives of the presented gates is generally not zero, the derivatives are lower than for naive gate implementations. For the optimal 18 ns gates the norm is around 0.8 instead of 10 for a simple rotation around one axis. These derivatives were calculated using dimensionless variables, with $\epsilon$ in units of $\epsilon_0$, and $J$ and $\Delta B_z$ in units of $J_0$. Our solutions do not constitute DCGs but decouple partly from slow noise. This can also be seen from their filter functions, which would be peaked at DC for free induction decay experiments but would be zero for decoupling sequences [11–14]. The (first-order) filter functions for the two 18-segment gates presented in the main text in Fig. 2 are given in panel (b) of Fig. S.4 and Fig. S.5. An additional gate, which rotates nearly around the z-axis ($\theta = 90°$), is given in Fig. S.6. The gates from the main text for $N_{\mathrm{seg}} = 30$ and $N_{\Delta B_z} = 3$ are given in figures Fig. S.7 and Fig. S.8, an additional gate for $\theta = 90°$ is shown in Fig. S.9. The filter functions of these gates are considerably lower as $\omega \to 0$ than at their peak but still finite. Hence, the gates are less sensitive to lower frequencies than high-frequency noise but do not decouple from slow noise completely.

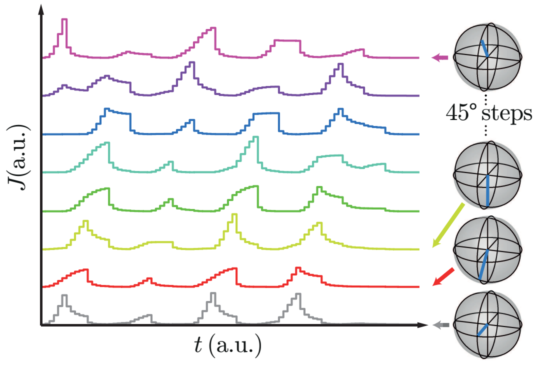


FIG. S.3. Pulse sequences for $\pi/2$-gates ($N_{\Delta B_z} = 4, N_{\mathrm{seg}} = 18$) are depicted for different axes. The axes were obtained by rotating the negative $y$-axis in steps of 45° around the idle-axis. Results are offset for clarity. For each sequence, $J$ is pulsed after the state vector has rotated by approximately $2\pi$. Furthermore, the phase of the pulses is obviously linked to the rotation axis, similar to Rabi driving.

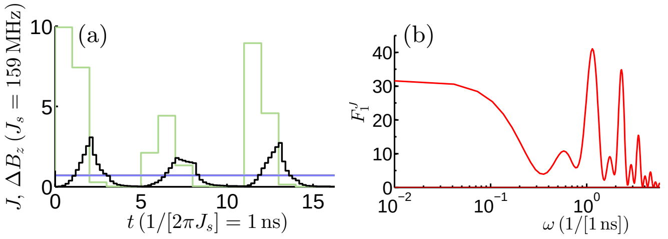


FIG. S.4. $\pi/2_x$-gate, $N_{\mathrm{seg}} = 18$, $N_{\Delta B_z} = 2$, $\mathcal{I} = 1.5 \times 10^{-3}$ (a) Blue: $\Delta B_z$. Green: rectangular $J$-pulses. Black: rise times approximated as piecewise constant. (b) $F_1^J$ is the first-order filter function in $J$.

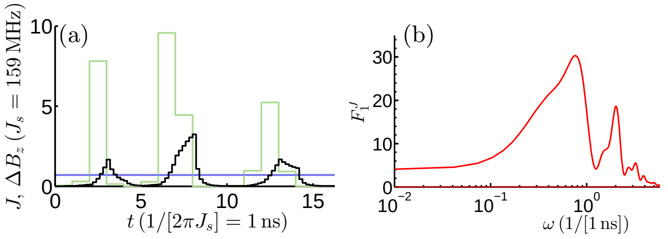


FIG. S.5. $\pi/2_y$, $N_{\mathrm{seg}} = 18$, $N_{\Delta B_z} = 2$, $\mathcal{I} = 1.6 \times 10^{-3}$

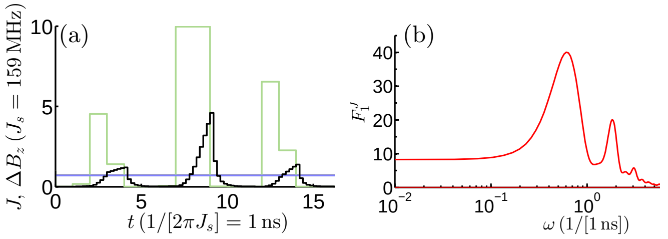


FIG. S.6. $\pi/2$-gate for $\theta = 90°$, $N_{\mathrm{seg}} = 18$, $N_{\Delta B_z} = 2$, $\mathcal{I} = 2.1 \times 10^{-3}$. The rotation axis of this gate lies close to the $z$-axis. $\theta$ describes the location of the rotation axis in the idle plane as defined in the text.

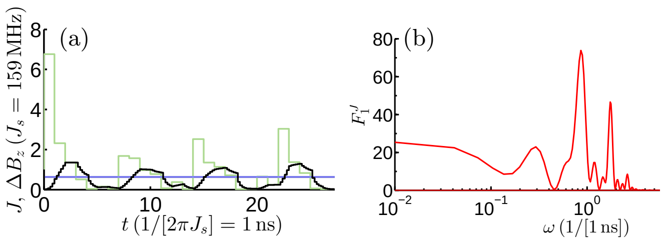


FIG. S.7. $\pi/2_x$,$N_{\mathrm{seg}} = 30$, $N_{\Delta B_z} = 3$, $\mathcal{I} = 1.1 \times 10^{-3}$

### H. Further solutions

Fidelities of the best solutions found for different parameters $N_{\mathrm{seg}}$ and $N_{\Delta B_z}$ for $\pi/2_y$-gates (around the negative $y$-axis) are shown in Fig. S.10. All of these qualitatively resemble the solutions for $\pi/2_x$-gates, which were dealt with in the main text (Fig. 3). We do not present solutions for $\pi$-gates here, because these are quite similar to the solutions for $\pi/2$-gates and similarly feature high fidelities.

As expected, gates have higher fidelities for more $N_{\mathrm{seg}}$. The added degrees of freedom allow better decoupling in both slow charge and hyperfine noise. This is illustrated in Fig. S.11 for $\pi/2_x$-gates, where the matrix 2-norm of the first-order derivatives $|dU/d\epsilon|$ and $|dU/d\Delta B_z|$ decreases for higher $N_{\mathrm{seg}}$.

### I. Noise contributions

As can be seen from Fig. S.12 the main contribution to the infidelity comes usually from fast noise in $\epsilon$ (except for the corner solutions), which is not significantly reduced for more $N_{\mathrm{seg}}$. For a more detailed comparison we also list the different infidelity contributions in Tab. S.1, exemplary for one gate.

The effect of fast noise is directly related to the amplitude of the exchange pulses which becomes clear when comparing the solutions for $N_{\mathrm{seg}} = 12$ and different $N_{\Delta B_z}$ in Fig. S.11 (c) and Fig. S.12 (b). For the corner solutions with $N_{\Delta B_z} = 1$ or $N_{\mathrm{seg}} = 12$ quasistatic contributions are dominant due to lower decoupling, as seen from the higher derivatives in Fig. S.11. Higher amplitude exchange pulses are used to implement decoupling properties when $N_{\mathrm{seg}}$ is high enough, but this leads to a higher adverse effect of fast charge noise.

### J. Gate robustness to model errors

The presented gates are rather insensitive to errors in parameter estimates of $J_0$, $\epsilon_0$ and $\tau_{\mathrm{rise}}$ or to offsets in the control parameters $\delta\epsilon$ and $\delta\Delta B_z$. The latter might be caused by calibration errors but also by quasistatic noise. We now look at the gate robustness exemplary for the gate shown in Fig. S.4 with $U_t = \pi/2_x$, $N_{\mathrm{seg}} = 18$ and $N_{\Delta B_z} = 2$.

For offsets $\delta\epsilon$ and $\delta\Delta B_z$ as large as $\pm 10\sigma_\epsilon$ and $\pm 5\sigma_{\Delta B_z}$, the infidelity from noise only deteriorates to $6.2 \times 10^{-3}$ as seen in Fig. S.13 (c). For offsets in $\delta\epsilon$, decoupling in $\Delta B_z$ is less pronounced, making hyperfine noise the dominant contribution to the deteriorated fidelity as seen in the line cut in panel (a). For $\delta\epsilon > 0$ the higher exchange coupling lead also to an increase of the contribution of high-frequency $\epsilon$-noise for both gates. Offsets in the hyperfine gradient destroy decoupling in $\epsilon$, as shown in (b), and have no effect on fast noise. The color plot in panel (c) provides the additional information that faster precession from a higher $\epsilon$ is partly compensated by lower $\Delta B_z$ (and vice versa). This holds for both the unitary and noise components of the infidelity. Comparing panel (c) and (d) one can see that the noise properties of the gate are especially insensitive to offsets in the parameters while systematic errors grow much faster.

Fig. S.14 (d) shows that if both $\epsilon_0$ and $J_0$ are overestimated (or both underestimated) the infidelity from noise

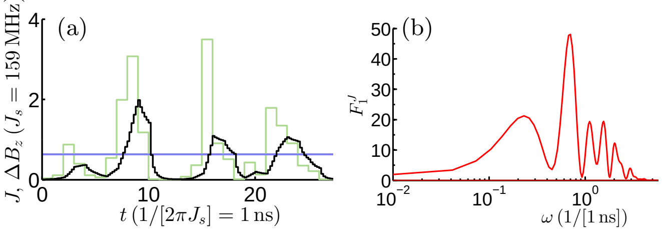


FIG. S.8. $\pi/2_y$, $N_{\mathrm{seg}} = 30$, $N_{\Delta B_z} = 3$, $\mathcal{I} = 0.9 \times 10^{-3}$

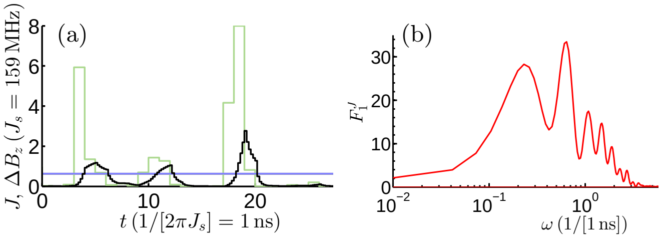


FIG. S.9. $\pi/2$, $\theta = 90°$, $N_{\mathrm{seg}} = 30$, $N_{\Delta B_z} = 3$, $\mathcal{I} = 1.0 \times 10^{-3}$

is only changed very little, as expected from the exponential model for $J(\epsilon)$. We only show infidelities from noise as systematic errors caused by wrong parameter estimates can be removed self-consistently by running the calibration routine. For the presented gate, simultaneous parameter errors as high as 20 % lead to infidelities of around $4.5 \times 10^{-3}$. The fidelity deterioration originates mainly from hyperfine and fast charge noise. In panel (c) we take a look at how noise properties change if rise times are different from 1 ns by ±20 % which only degrades the infidelity to maximally $3.5 \times 10^{-3}$. Again, dominant contributions stem from fast $\epsilon$- and slow $\Delta B_z$-noise. Lower rise times increase the effect of fast charge noise because pulses saturate faster and are hence able to reach higher $J$. Furthermore, decoupling in $\Delta B_z$ is less pronounced, making hyperfine noise a major contributing factor.

Overall, the above discussion suggests that the presented gate is sufficiently impervious to model errors if one aims for gates with fidelities > 99 %, assuming systematic errors can be tuned away.

To easily assess how robust the other numerical solutions are with respect to model errors, we condense all of the above information into a single figure of merit $\mathcal{I}_{\mathrm{worst}}$. In order to calculate this quantity, we calculate the maximum infidelity from noise for simultaneous errors in $J_0$ and $\epsilon_0$ of ±20 %, taking the worst combination of the two from the color plot (d) in Fig. S.14. Additionally, we extract the worst infidelity from noise for wrong rise times in the range of ±20 %, which corresponds to the maximum in panel (c). The ranges of ±20 % were chosen as very wide confidence bounds for the experimental reality. The proxy for the sensitivity of a gate to these errors is then defined as

$$\mathcal{I}_{\mathrm{worst}} = \sqrt{(\mathcal{I}_{\mathrm{worst},\, J_0,\, \epsilon_0})^2 + (\mathcal{I}_{\mathrm{worst},\, \tau_{\mathrm{rise}}})^2}, \qquad \text{(S.4)}$$

TABLE S.1. Infidelity contributions with Monte Carlo (1000 time traces) and fast method for the gate shown in Fig. S.4 ($U_t = \pi/2_x$, $N_{\mathrm{seg}} = 18$, $N_{\Delta B_z} = 2$). The fast method is only slightly less accurate, well within other uncertainties of the simulation, but speeds up calculation by at least a factor $10^3$.

| | Monte Carlo | Fast Method | Abs. Δ | Rel. Δ |
|---|---|---|---|---|
| $\mathcal{I}_{\epsilon,\mathrm{fast}}$ | $9.98 \times 10^{-4}$ | $9.36 \times 10^{-4}$ | $3.8 \times 10^{-5}$ | 5 % |
| $\mathcal{I}_{\epsilon,\mathrm{slow}}$ | $3.50 \times 10^{-4}$ | $3.43 \times 10^{-4}$ | $-0.6 \times 10^{-5}$ | −2 % |
| $\mathcal{I}_{\Delta B_z}$ | $2.68 \times 10^{-4}$ | $2.64 \times 10^{-4}$ | $-0.3 \times 10^{-5}$ | −1 % |
| $\mathcal{I}_U$ | $1.35 \times 10^{-13}$ | $1.35 \times 10^{-13}$ | | |
| $\mathcal{I}$ | $1.52 \times 10^{-3}$ | $1.54 \times 10^{-3}$ | $3 \times 10^{-5}$ | 2 % |

and is plotted in panels (b) of Fig. S.10 and Fig. 3. One can see that especially solutions with $N_{\Delta B_z} = 1$ and large $N_{\mathrm{seg}}$ are unattractive.

## K. Numerical analysis

Having presented the results produced by the algorithm used for fidelity optimization in the last sections, we will now evaluate the algorithm's performance. We will first explain features observed in convergence plots and then present evidence that indeed the solution with the highest possible fidelity was found.

Typical convergence plots are shown in Fig. S.15 (a) and (b). These are representative of the convergence behavior observed in numerous other optimization runs. Iterations were stopped after the count of 400. The initial steep convergence is a feature of the Gauss-Newton algorithm (GNA) part of the Levenberg-Marquardt algorithm (LMA) and is mainly produced by eliminating systematic errors within the first 10 to 20 iterations [15, 16]. The rest of the iteration time is spent on optimizing the noise properties. This can be observed in Fig. S.15 (c), where the dashed lines on the left are orders of magnitude lower than the other components. That systematic errors are removed first is owed to the construction of the objective function as discussed previously in Sec. I C.

Usually the solver succeeds in lowering the contribution to the infidelity from the systematic gate error to $10^{-10}$ or lower, which for practical purposes represents no systematic errors. It is reasonable that for enough degrees of freedom perfect gate implementations exist, as arbitrary rotations around two axes are enough to reach each point on the Bloch sphere. Yet, it seems unlikely that the gate can be made completely resistant to fast and slow noise. Therefore, systematic errors approach zero while the infidelity from noise does not.

Once systematic errors have been removed to a high degree, the solver focuses on the pulse's noise properties. As can be seen from the systematic infidelity in Fig. S.15 (c), the search direction changes in between. The zigzags correspond to changes in the LMA's damping pa-

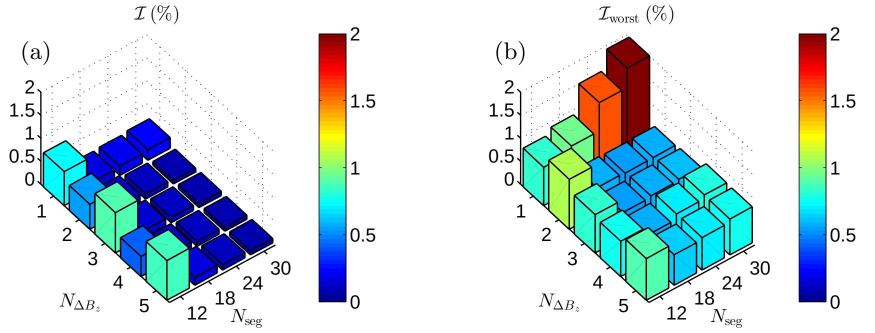


FIG. S.10. (a) Best solutions for $\pi/2_y$-gates for different number of pure $\Delta B_z$-rotations and number of $\epsilon$-pulses. (b) Maximum deterioration of the infidelity (only considering the contributions from noise) for model errors in $J_0$, $\epsilon_0$ and $\tau_{\text{rise}}$ as large as 20%.

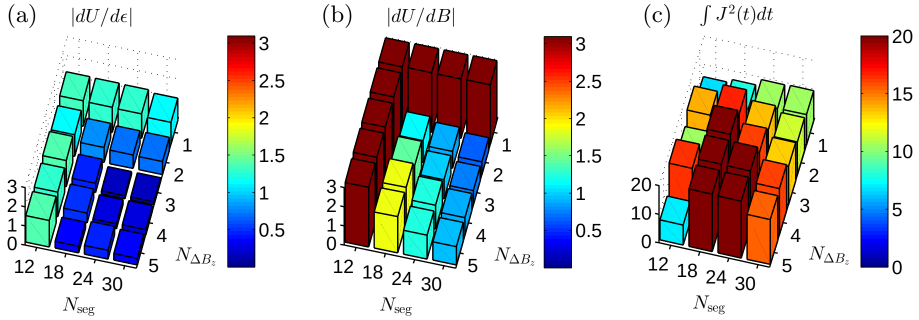


FIG. S.11. Matrix 2-norm of the derivatives of the unitary time evolution operators of $\pi/2_x$-gates (a) with respect to $\Delta B_z$ and (b) with respect to $\epsilon$. Values higher than 3 were cut off. (c) $\int J^2 dt$ serves as a proxy for the amplitude of the exchange pulses. Values higher than 20 were cut off.

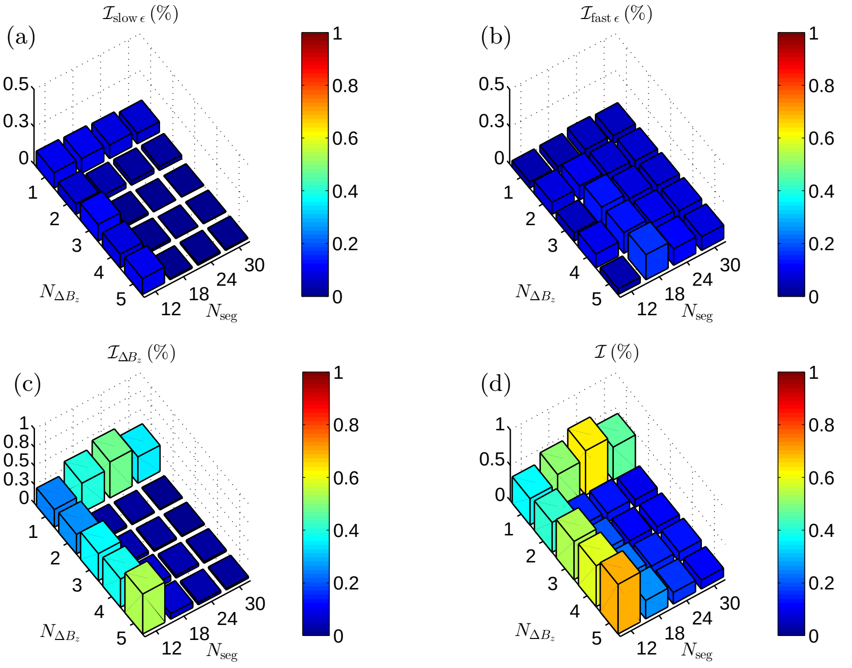


FIG. S.12. Contributions to $\mathcal{I}$ of the $\pi/2_x$-gates from (a) slow and (b) fast charge noise and (c) hyperfine noise. (d) Total $\mathcal{I}$.

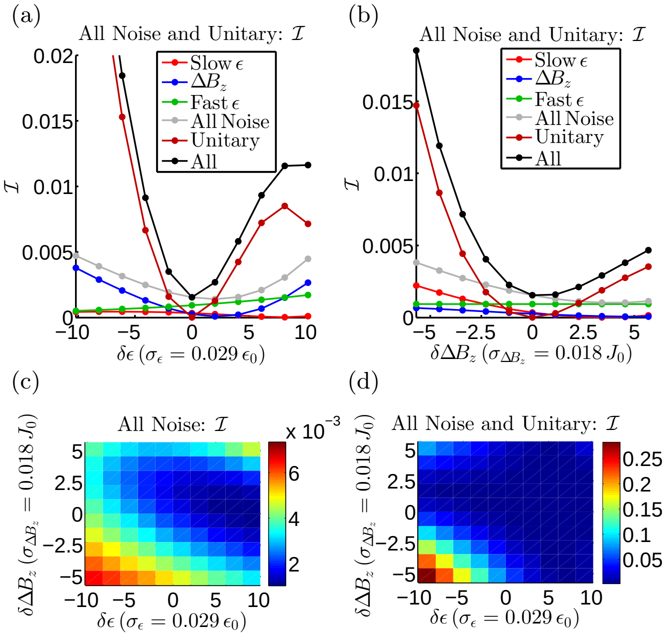


FIG. S.13. Robustness of the gate shown in Fig. S.4 with respect to offsets in $\epsilon$ and $\Delta B_z$, measured in units of the total noises' standard deviations. Generally, the infidelity is dominated by systematic errors. (a) Line cut for $\delta\epsilon$ and (b) for $\delta\Delta B_z$, where systematic (unitary) errors increase quite quickly. (c) The effect on the infidelity only from noise is relatively low. (d) The effect on the infidelity from noise and systematic deviations.

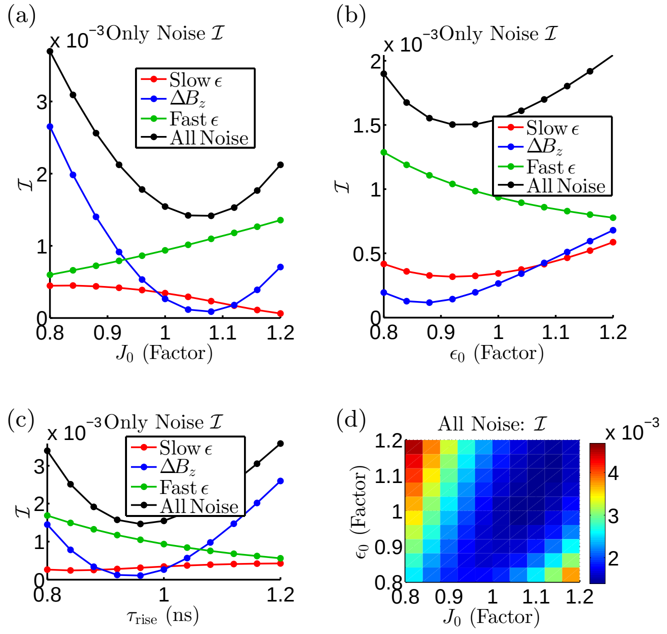


FIG. S.14. Robustness of the gate shown in Fig. S.4 with respect to errors in the model $J(\epsilon)$ for the parameters $J_0$ and $\epsilon_0$. The gate's robustness to large errors is relatively high. (a) Line cut for $J_0$, (b) for $\epsilon_0$ and (c) the rise time $\tau_{\text{rise}}$. The effect on the infidelity from noise is relatively low. (d) The effect on the infidelity from noise and systematic deviations. If $\epsilon_0$ is too high, $\epsilon$ is lower than expected, which is compensated if $J_0$ is also too high.

rameter, where the solver moves more to the gradient descent direction because the GNA no longer provides sufficient improvements. In the right subfigure, one can observe that the effect of fast noise (solid line) increases in the beginning, as low starting values in $\epsilon$ are increased to implement the target gate. At the same time, decoupling in the slow components (dashed and dotted) is increased. Thus, the infidelities from the different noise contributions converge towards one another, as expected from minimizing their sum of squares.

The slow creep after the initial fast convergence goes on for much longer than 400 iterations, eventually leading to only minuscule improvements (we checked this up to 2500 iterations). It is therefore sufficient to stop after 400 iterations but we note that more iterations would be beneficial for larger $N_{\text{seg}}$ than considered in this work.

Other optimization algorithms could be more suitable for this specific task and speed up the slow creep after the initial fast convergence. However, trying different algorithms (including derivative-free methods) we found that the LMA showed the highest convergence speed and found the best solutions. Actually finding the best solution is more important for this work than speed of convergence.

In order to assess whether the optimization managed to find the best solution (with the highest fidelity), we look

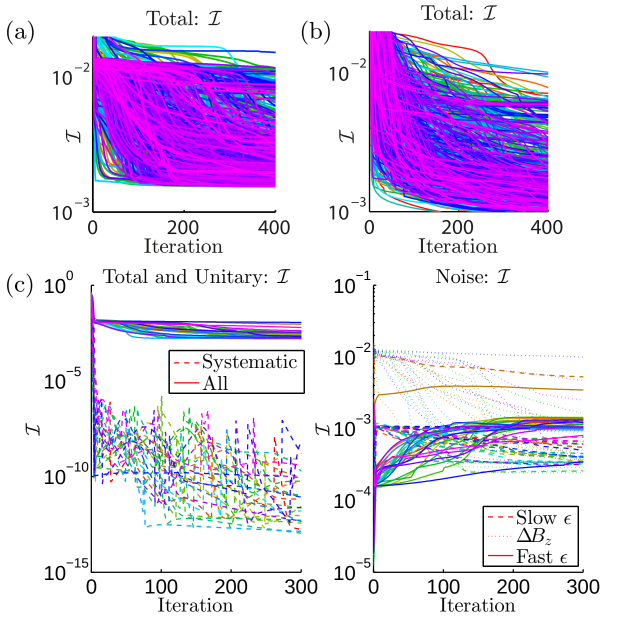


FIG. S.15. LMA convergence for 1000 runs of the (a) 18-segment gate from Fig. S.4 and of the (b) 30-segment gate from Fig. S.7. The bigger parameter space leads to slower convergence for some of the runs. (c) Infidelity components for 25 runs of the 18-segment gate.

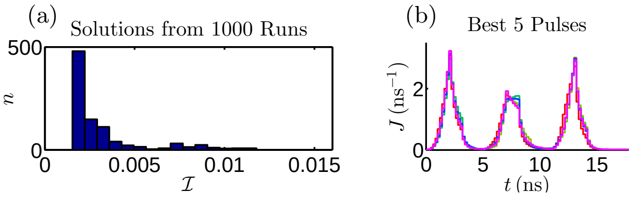


FIG. S.16. Uniqueness of solutions for the 18-segment gate from Fig. S.4. (a) Histogram of $\mathcal{I}$ achieved in all runs (very high $\mathcal{I}$ not shown). (b) The overlay of pulse shapes of the best 5 solutions suggests good convergence.

at the 5 best solutions obtained for one run with 1000 different random starting values and plot a histogram of the infidelities of all solutions (from one run). These plots are shown for $N_{\rm seg} = 18$ in Fig. S.16. Panel (a) shows that many solutions with similiar performance are found. Furthermore, panel (b) illustrates that the optimization algorithm actually manages to find the best numerical solution several times (with some negligible deviations). As long as one is willing to assume that the best numerical simulation's convergence radius can serve as a proxy for the best solution's convergence radius, this indicates sufficient coverage of parameter space. Slight variations in the pulse shapes, which increase in the number of free parameters, could be removed in further iterations but as mentioned before this would only lead to minuscule fidelity improvements.

In summary, convergence could still be improved but is sufficient for finding very high-fidelity gates. From the above analysis it seems reasonable to conclude that for practical purposes the numerical solutions have converged to the best solution. Any relative fidelity improvements below 10 % are well within other uncertainties of the model due to imperfectly characterized $J_0$, $\epsilon_0$ and $\tau_{\rm rise}$.

## II. SELF-CONSISTENT CALIBRATION ROUTINE

In addition to the $\pi/2_x$- and $\pi/2_y$-gates with 18 segments, we also benchmarked the other gate set mentioned in the main text with 30 segments ($N_{\Delta B_z} = 3$). The performance shown in Fig. S.17 is quite similar to the one presented in Fig. 4.

### A. Choice of weights

The problem given in Eq. 3 is very similar to the numerical gate search since the infidelity due to systematic errors $\mathcal{I}_s$ scales as $|\boldsymbol{S}|^2$. Therefore, $\mathcal{I}_s$ will be smaller than the infidelity from noise $\mathcal{I}_n$ when the calibration routine has converged. However, different weights $w_n, w_n'$ can be used to adjust the relative importance that the calibration routine ascribes to systematic errors in comparison

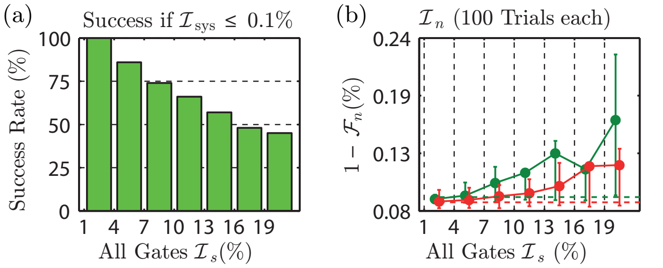


FIG. S.17. Convergence of the self-consistent tuning protocol for the gate set consisting of a $\pi/2_x$- and a $\pi/2_y$-gate ($N_{\rm seg} = 30, N_{\Delta B_z} = 3$) with a similar performance as the set used in the main text. (a) Success rate for initial infidelities $\mathcal{I}_s$. (b) Infidelity from noise $\mathcal{I}_n$ of the final calibrated gates (dots) and of the perfect gates (dashed lines). Error bars show the 10th and 90th percentile of the distribution of $\mathcal{I}_n$ over 100 runs per bin for different starting gates.

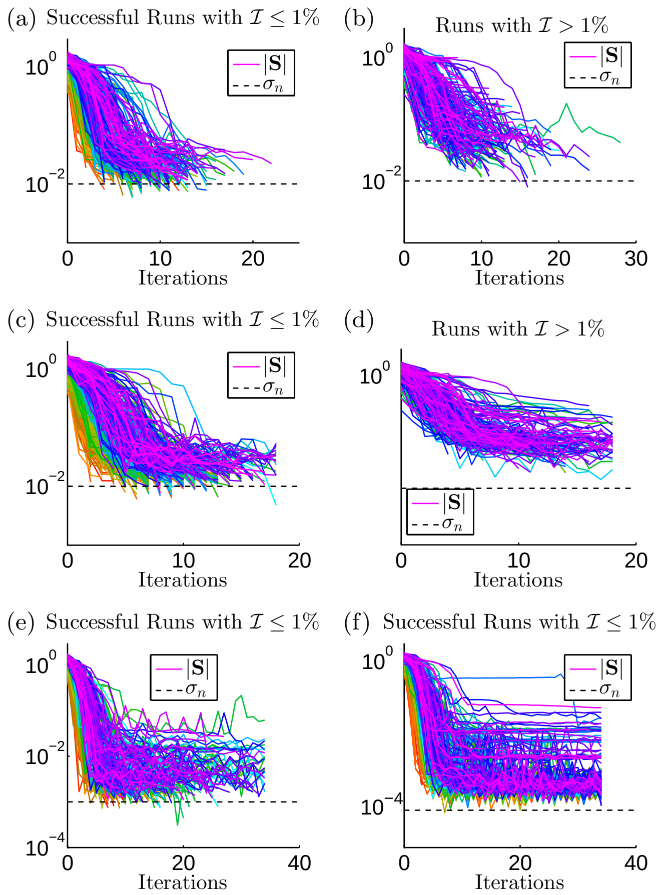


FIG. S.18. Calibration protocol convergence for different gate sets and noise levels (indicated by the black dashed line). (a) Successful and (b) unsuccessful runs of the 18-segment gate set. (c) Successful and (d) unsuccessful runs of the 30-segment gate set. Some of the unsuccessful trials reach quite low $|\boldsymbol{S}|$ but do not succeed in retaining the pulses' noise properties. (e) Successful runs for the 18-segment pulses for $\sigma_S = 10^{-3}$ and (f) $\sigma_S = 10^{-4}$.

to decoherence. To find values for $w_n$ and $w'_n$ which achieve good convergence, we start by making the problem symmetric and choose

$$w_n = v_n \frac{\sqrt{\mathcal{I}_{s,t}}}{\mathcal{I}_{n,t}}, \tag{S.5}$$

$$w'_n = v_n \frac{\sqrt{\mathcal{I}_{s,t}}}{\mathcal{I}'_{n,t}}. \tag{S.6}$$

Here, $v_n$ is a new heuristically chosen weight and $\mathcal{I}_{s,t}$ describes the reachable target infidelity for systematic errors when considering measurement noise (as discussed below). $\mathcal{I}_{n,t}$ and $\mathcal{I}'_{n,t}$ are the infidelities from noise of the perfect gates. With this formulation, the contributions of $w_n\mathcal{I}_n(\boldsymbol{\epsilon})$ and $w'_n\mathcal{I}_n(\boldsymbol{\epsilon})$ will be on the same order as $\sqrt{\mathcal{I}_{s,t}}$ if the calibration routine succeeded in retrieving the perfect gate. We tried different values for the weight $v_n$ and found that for $1 \leq v_n \leq 10$ the algorithm converged most often.

We also added a feature which significantly increases the solver's convergence for a wide variety of low-fidelity starting values. If the algorithm fails to converge for a certain gate set, a new trial is started with increased weights $v_n$. Initially we choose $v_n = 1$. We optimized the algorithm by hand and found $v_n \in \{1, 3, 5, 7\}$ to provide robust convergence with a low number of trials. If the algorithm does not succeed with $v_n = 7$, it fails altogether for a specific set of starting values.

### B. Measurement noise

The above discussion did not take the measurement process which is used to extract the signals $S_i$ into account. Repeated single shot readout of the (same) qubit state can be used to measure the projection of the state vector along the $z$-axis with high fidelity [7, 17, 18]. The same final state can be prepared multiple times by repeatedly initializing the qubit to $|0\rangle$ and applying the same pulse sequence $i$.

More repetitions lead to a smaller uncertainty in the measurement. For $n$ single shot measurements, the probability mass function for obtaining $k$ triplet outcomes follows a binomial distribution with triplet probability $p_T$. For big $n$ this is well approximated by a Gaussian distribution $N(np_t, np_t[1-p_t])$. Averaging over these measurements then gives the signal $S_i$, which is also transformed linearly to lie between $-1$ and 1 (the eigenvalues of $\sigma_z$). The resulting signal is distributed as $N(2p_t - 1, 4p_t[1-p_t]/n)$. Since the calibration protocol pulses end up on or close to the equatorial plane, $p_T \approx 1/2$ for sufficiently good gates. Therefore, $n \approx 1/\sigma_S^2$ measurements are needed to achieve an accuracy $\sigma_S$. Below this accuracy, measured signals vary randomly.

Every single shot measurement takes on the order of 1 µs. The main contributing factor is averaging over the current signal of the quantum point contact, which is used to readout the qubit's charge state via spin to charge conversion. The number $n$ of single shot measurements performed by the algorithm in each iteration is given as

$$n \approx \frac{(2N_{\text{dof}} + 1)N_{\text{signals}}}{\sigma_S^2}, \tag{S.7}$$

where $N_{\text{dof}} = 2(N_{\text{seg}} - 4)$ denotes the degrees of freedom the solver can adjust (4 segments at the end of each of the two pulses are fixed to $\epsilon_{\text{min}}$ to avoid transients) and $N_{\text{signals}} = 6$ is the number of pulse sequences. The term $2N_{\text{dof}}$ includes the measurements needed to calculate the Jacobian using central differences. While the pure measurement time is below 2 s (for $\sigma_S = 10^{-2}$ and $N_{\text{seg}} = 18$), a pulse update on the AWG takes much longer (about 2 min for the Tektronix AWG 5000 series).

For a randomly fluctuating objective function $\boldsymbol{S}$, using the LMA with finite differences leads to problems for small step sizes $h$ in $\epsilon$ because the numerical derivative is likely to be dominated by statistical fluctuations. We remedy this problem by setting a lower bound $h_{\text{min}} = 0.3\epsilon_0$ which we found to yield good results for $\sigma_S = 10^{-2}$. Too low a bound leads to erratic behavior of the solver, while too high a bound also hinders convergence if $h_{\text{min}}$ is much bigger than the width of a minimum in the landscape of the objective function.

### C. Convergence

The convergence behavior of the calibration routine is very similar to the gate search. This is expected because the same optimization algorithm was used on two very similar problems. Initial convergence is fast as before but eventually stops, when $|\boldsymbol{S}| \sim \sigma_S$ (Fig. S.18). To verify that convergence indeed depends on the noise level, we also performed simulations for $\sigma_S = 10^{-3}$ ($10^{-4}$). As expected, $\mathcal{I}_{\text{sys}}$ was usually on the order of $10^{-6}$ ($10^{-8}$). The convergence plots in Fig. S.18 (e) and (f) show how the algorithm is unable to go below the threshold set by the noise level. If no lower bound $h_{\text{min}}$ is set, the algorithm fails to converge most of the time with a success rate of about 10 % for initial $\mathcal{I}_s$ between 1 % and 4 %.

### D. Fidelity $\mathcal{I}_{\text{sys}}$

One indication of whether the calibration routine successfully removed systematic errors is $|\boldsymbol{S}|$. For an independent measure we also calculated the infidelity $\mathcal{I}_{\text{sys}}$ which only includes systematic errors. Since the calibration protocol is invariant under rotations around the measurement axis, we neglect the orientation of the rotation axes of both pulses in the $xy$-plane. To calculate $\mathcal{I}_{\text{sys}}$, we first project the rotation axis of the first pulse onto the $xy$-plane. The projected unitary $U_{t,1}$ rotates by an angle $\pi/2$ around this projected axis, and serves as the target unitary for the first pulse with $\mathcal{I}_{\text{sys}} = \mathcal{I}(U(\boldsymbol{\epsilon}, \Delta B_z), U_{t,1})$. The second pulse is compared with a target unitary $U_{t,2}$

which is obtained by rotating the rotation axis of $U_{t,1}$ by $\pm 90^\circ$ around the $z$-axis. $\mathcal{I}_{\mathrm{sys}}$ is just used to check whether a low $|\boldsymbol{S}|$ is compatible with the fidelity threshold for successful convergence of the calibration routine. Furthermore, the initial infidelity $\mathcal{I}_s$ of the imperfect pulses used as starting values for the calibration routine is calculated in this way.

### E. Setting the orientation of the rotation axes in the $xy$-plane

In order to tune a specific set of gates without any additional degrees of freedom, one would need to set the orientation of the pulses' rotation axes in the plane defined by the measurement and initialization axis. This can be done by executing the calibration routine as explained in the main text with the addition of one sequence $S_7$, which involves reading out along an axis orthogonal to the the old measurement axis. The choice of the orthogonal axis corresponds to choosing the in-plane orientation. For example, if measurement and initialization are performed along the $z$-axis, one could measure along the $x$-axis in addition (best done adiabatically as used by Foletti *et al.* [19]). Then, preparing the $|0\rangle$ state, applying a $\pi/2_x$-pulse and reading out along the $x$-axis fixes the rotation axis of this pulse to the $x$-axis. We tested this procedure in our numerical benchmarks and found that it does not impair the bootstrap performance significantly.


[1] T. J. Green, J. Sastrawan, H. Uys, and M. J. Biercuk, (2012), arXiv:1211.1163.

[2] T. Green, H. Uys, and M. J. Biercuk, Physical Review Letters **109**, 020501 (2012).

[3] O. E. Dial, M. D. Shulman, S. P. Harvey, H. Bluhm, V. Umansky, and A. Yacoby, Physical Review Letters **110**, 146804 (2013).

[4] R. Koch, J. Rozen, G. Keefe, F. Milliken, C. Tsuei, J. Kirtley, and D. DiVincenzo, Physical Review B **72**, 092512 (2005).

[5] H. Bluhm, S. Foletti, D. Mahalu, V. Umansky, and A. Yacoby, Physical Review Letters **105**, 216803 (2010).

[6] L. M. K. Vandersypen, **76**, 1037 (2004).

[7] C. Barthel, J. Medford, H. Bluhm, A. Yacoby, C. Marcus, M. Hanson, and A. Gossard, Physical Review B **85**, 035306 (2012).

[8] K. Khodjasteh and L. Viola, Physical Review A **80**, 032314 (2009).

[9] K. Khodjasteh and L. Viola, Physical Review Letters **102**, 080501 (2009).

[10] X. Wang, L. S. Bishop, E. Barnes, J. P. Kestner, and S. Das Sarma, Physical Review A **89**, 022310 (2014).

[11] J. Martinis, S. Nam, J. Aumentado, K. Lang, and C. Urbina, Physical Review B **67**, 094510 (2003).

[12] L. Cywinski, R. Lutchyn, C. Nave, and S. Das Sarma, Physical Review B **77**, 174509 (2008).

[13] M. J. Biercuk, H. Uys, A. P. VanDevender, N. Shiga, W. M. Itano, and J. J. Bollinger, Nature **458**, 996 (2009).

[14] M. Biercuk and H. Bluhm, Physical Review B **83**, 235316 (2011).

[15] K. Levenberg, Quarterly of Applied Mathematics **2**, 164 (1944).

[16] D. W. Marquardt, SIAM Journal on Applied Mathematics **11**, 431 (1963).

[17] C. Barthel, D. Reilly, C. Marcus, M. Hanson, and A. Gossard, Physical Review Letters **103**, 160503 (2009).

[18] C. Barthel, M. Kjærgaard, J. Medford, M. Stopa, C. Marcus, M. P. Hanson, and A. C. Gossard, Physical Review B **81**, 161308 (2010).

[19] S. Foletti, H. Bluhm, D. Mahalu, V. Umansky, and A. Yacoby, Nature Physics **5**, 903 (2009).
